# Supplementary material for: From Skew to Symmetry: Node-Interconnect Multi-Path Balancing with Execution-time Planning for Modern GPU Clusters
Source: arXiv:2604.00317 source file (2026-03-31)
Supplement: Supplementary file 1 [file 9-Appendix.tex]

\twocolumn[%
{\begin{center}
\Huge
Appendix: Artifact Description/Artifact Evaluation        
\end{center}}
]

%%%%%%%%%%%%%%%%%%%%%%%%%%%%%%%%%%%%%%%%%%%%%%%%%%%%%
%  AD Appendix
%%%%%%%%%%%%%%%%%%%%%%%%%%%%%%%%%%%%%%%%%%%%%%%%%%%%%

\appendixAD

\section{Overview of Contributions and Artifacts}

\subsection{Paper's Main Contributions}

\begin{description}
\item[$C_1$] We propose \textbf{NIMBLE}, a novel runtime system designed to dynamically mitigate communication skew in heterogeneous HPC systems by intelligently redistributing traffic across all available links. NIMBLE operates transparently and is application-agnostic.
\item[$C_2$] We design an \textbf{adaptive load balancing algorithm}, inspired by multi-commodity flow (MCF) principles but adapted for runtime efficiency, that computes near-optimal data redistribution strategies across diverse intra-node (e.g., NVLink) and inter-node (e.g., InfiniBand/RoCE, considering rail affinity) paths based on dynamic link utilization.
\item[$C_3$] We develop a \textbf{CUDA-aware, kernel-based pipelining mechanism} for efficient, low-overhead multi-hop data forwarding via intermediate GPUs and NICs, enabling non-blocking transfers essential for exploiting redistributed communication paths.
\item[$C_4$] We ensure NIMBLE \textbf{integrates seamlessly} with existing communication libraries like NCCL, requiring \textbf{no modifications to user application code} and introducing negligible overhead for the orchestration logic compared to communication latency.
\item[$C_5$] We demonstrate through evaluation that \textbf{NIMBLE} significantly improves performance for communication-skewed workloads, achieving up to \textbf{2x and 3.4x throughput speedups} over state-of-the-art baselines in All-to-Allv and irregular Send/Recv applications, respectively. 
\end{description}

\subsection{Computational Artifacts}

\begin{description}
\item[$A_1$] https://doi.org/10.5281/zenodo.18672256
\end{description}

\begin{center}
\begin{tabular}{rll}
\toprule
Artifact ID  &  Contributions &  Related \\
             &  Supported     &  Paper Elements \\
\midrule
$A_1$   &  $C_{1,2,3,4,5}$ & Figure 6,7 \\
\bottomrule
\end{tabular}
\end{center}

%%%%%%%%%%%%%%%%%%%%%%%%%%%%%%%%%%%%%%%%%%%%%%%%%%%%%%%%
\section{Artifact Identification}
%%%%%%%%%%%%%%%%%%%%%%%%%%%%%%%%%%%%%%%%%%%%%%%%%%%%%%%%

\newartifact

\artrel

Artifact $A_1$ is the implementation and microbenchmark used to evaluate \textbf{NIMBLE}.
It contains prebuilt baseline communication libraries (\texttt{nccl\_build}) and a NIMBLE-enabled build (\texttt{nimble\_build}), together with a standalone benchmark (\texttt{benchmark.cc}) and launcher script (\texttt{run.sh}).
The artifact supports contributions $C_{1}$--$C_{4}$ by providing the NIMBLE runtime integrated into an NCCL-like API, and supports $C_{5}$ by reproducing the performance trends shown in Figure~\ref{fig:four_figures} and Figure~\ref{fig:skew_bw}.

\artexp

We expect NIMBLE to achieve higher effective bandwidth than the baseline when the communication pattern is (i) bottlenecked on a subset of links and/or (ii) sufficiently large to benefit from multi-path pipelining.
Specifically:
\begin{itemize}
    \item \textbf{Figure~\ref{fig:four_figures} (point-to-point / \texttt{--p2p}):} NIMBLE should outperform the baseline by utilizing additional intra-node NVLink links (via intermediate GPUs) and additional inter-node NIC rails (via GPU--NIC forwarding). On our evaluation system, NIMBLE reaches up to 278.2~GB/s intra-node peak bandwidth with two intermediates and up to 170.0~GB/s inter-node peak bandwidth with four NICs, while direct paths saturate at lower throughput.
    \item \textbf{Figure~\ref{fig:skew_bw} (skewed all-to-allv / \texttt{--skewed}):} as the hotspot ratio increases, NIMBLE should provide increasing speedup by rerouting traffic away from congested links. In the paper's evaluation, when the hotspot ratio reaches 0.7 or higher, NIMBLE is up to 5.2$\times$ faster than NCCL for large messages.
\end{itemize}
These outcomes substantiate $C_1$--$C_3$ (adaptive multi-path planning + low-overhead forwarding) and $C_5$ (end-to-end speedup on skewed workloads).

\artin

\artinpart{Hardware}

\begin{itemize}
    \item \textbf{Tested platform (paper):} 2 nodes; each node has 4$\times$ NVIDIA H100 (SXM5, NVLink~4) and 4$\times$ NDR400 InfiniBand HCAs (one HCA per GPU) with GPUDirect RDMA.
    \item \textbf{Minimum to run the benchmark:} at least 1 node with 2 CUDA-capable GPUs (or 2 visible GPUs) to run \texttt{--p2p} intra-node.
    \item \textbf{To reproduce Figure~\ref{fig:four_figures} and Figure~\ref{fig:skew_bw}:} multi-GPU NVLink intra-node fabric and at least 2 nodes connected by an RDMA-capable interconnect (InfiniBand or RoCE) are required; for the full inter-node multi-rail results, multiple NICs/rails per node are required.
\end{itemize}

\artinpart{Software}

\begin{itemize}
    \item \textbf{Operating system:} Linux (HPC environment).
    \item \textbf{CUDA toolkit:} CUDA~12.x (tested with CUDA~12.6.2). \url{https://developer.nvidia.com/cuda-toolkit}
    \item \textbf{MPI:} Open MPI~5.x (tested with Open~MPI~5.0.7). \url{https://www.open-mpi.org/}
    \item \textbf{Communication libraries (included in the artifact):}
    baseline NCCL and a NIMBLE-enabled build (built from the same codebase; the distributed headers report NCCL~2.23.4). NCCL: \url{https://developer.nvidia.com/nccl}
    \item \textbf{Artifact entry point:} \texttt{run.sh} (compiles \texttt{benchmark.cc} with \texttt{mpicxx} and runs it with \texttt{mpirun}).
\end{itemize}

%%%%%%%%%%%%%%%%%%%%%%%%%%%%%%%%%%%%%%%%%%%%%%%%%%%%%
%  AE Appendix
%%%%%%%%%%%%%%%%%%%%%%%%%%%%%%%%%%%%%%%%%%%%%%%%%%%%%
\newpage
\appendixAE

\arteval{1}
\artin

\artinpart{Datasets / Inputs}

No external datasets are required. Workloads are generated deterministically at runtime (fixed RNG seed).
Inputs are:
\begin{itemize}
    \item an Open~MPI hostfile path (\texttt{--hostfile})
    \item number of MPI ranks (\texttt{--np})
    \item benchmark parameters: message size in MB (\texttt{size\_mb}, positional), hotspot ratio (\texttt{ratio}, positional, only for \texttt{--skewed}), and flags (\texttt{--p2p}, \texttt{--skewed}, etc.)
\end{itemize}

\artinpart{Installation and Deployment}

\begin{enumerate}
    \item Download and extract the artifact from $A_1$ (Zenodo DOI above).
    \item \textbf{From the artifact root}, enter the benchmark directory:
    \begin{verbatim}
cd ipdps_adae
    \end{verbatim}
    \item Export required environment variables (validated by \texttt{run.sh}):
    \begin{verbatim}
export CUDA_HOME=/path/to/cuda
export OMPI_HOME=/path/to/openmpi
    \end{verbatim}
    \item Ensure \texttt{nccl\_build/} and \texttt{nimble\_build/} are present (prebuilt libraries). No library rebuild is needed for the artifact evaluation.
    \item Prepare a hostfile matching the desired placement (examples are given below). Then run \texttt{run.sh}.
\end{enumerate}

\artcomp

\textbf{Workflow overview:}
\vspace{0.5ex}
\textbf{Experiment parameters and how they map to the paper:}
\begin{itemize}
    \item \textbf{Build selection (baseline vs.\ NIMBLE):} use \texttt{--no-nimble} and \texttt{--nimble} to select \texttt{nccl\_build} or \texttt{nimble\_build}, respectively.
    \item \textbf{Figure~\ref{fig:four_figures} (Figure 6) -- point-to-point:} run the benchmark with \texttt{--p2p} to create a single non-zero transfer in the all-to-all payload matrix. Sweep \texttt{size\_mb} to obtain bandwidth curves. To expose more intra-node GPUs / inter-node NICs as forwarding resources, increase ranks per node (e.g., 2/3/4 ranks on one node; 1--4 ranks per node on two nodes).
    \item \textbf{Figure~\ref{fig:skew_bw} (Figure 7) -- skewed all-to-allv:} run with \texttt{--skewed} and set the hotspot ratio via the second positional argument (e.g., 0.4--1.0). The paper uses 8~GPUs across two nodes (4~ranks per node); use \texttt{--np 8} and a 2-node hostfile with 4 slots per node.
    \item \textbf{Repetitions/statistics:} each run performs 5 warmup rounds and reports statistics over 100 timed rounds. For additional stability, repeat each configuration 3 times and report the median.
\end{itemize}

\vspace{0.5ex}
\textbf{Command examples (run from \texttt{ipdps\_adae}):}
(\textit{Note:} also provide \texttt{--hostfile <HOSTFILE>} and \texttt{--np 8} to \texttt{run.sh}.)
\begin{itemize}
    \item Show help:
    \begin{verbatim}
./run.sh -h
    \end{verbatim}
    \item Figure~\ref{fig:four_figures} (p2p, baseline vs.\ NIMBLE; 8 ranks / 2 nodes):
    \begin{verbatim}
--no-nimble -- 256 --p2p
--nimble   -- 256 --p2p
    \end{verbatim}
    \item Figure~\ref{fig:skew_bw} (skewed, hotspot ratio 0.7; 8 ranks / 2 nodes):
    \begin{verbatim}
--no-nimble -- 256 0.7 --skewed
--nimble   -- 256 0.7 --skewed
    \end{verbatim}
\end{itemize}
Example hostfile contents (edit node names to match your allocation):
\begin{verbatim}
node0 slots=4
node1 slots=4
\end{verbatim}

\artout

\begin{itemize}
    \item Use rank~0 \texttt{Peak Bandwidth} (GB/s) as the primary metric and compute speedup as BW(\texttt{--nimble})/BW(\texttt{--no-nimble}).
    \item Figure~\ref{fig:four_figures}: sweep \texttt{size\_mb}; NIMBLE should improve bandwidth, especially at larger message sizes.
    \item Figure~\ref{fig:skew_bw}: sweep hotspot \texttt{ratio} (e.g., 0.4--1.0); speedup should increase as \texttt{ratio} increases.
    \item (Optional) Check \texttt{alltoall\_payload\_volume.txt} to confirm the intended traffic pattern (\texttt{--p2p} vs.\ \texttt{--skewed}).
\end{itemize}
